# Supplementary material for: Collective magnetism of atomic momentum states
Source: arXiv:2502.09293 ancillary file (2025-02-13)
Supplement: Supplementary file 1 [file sm.pdf]

# Supplement: Collective magnetism of atomic momentum states

Garrett R. Williams,<sup>1</sup> Rishi P. Lohar,<sup>1</sup> Tao Chen,<sup>1</sup> Brian L. DeMarco,<sup>1,\*</sup> and Bryce Gadway<sup>1,2,†</sup>

<sup>1</sup>*Department of Physics, University of Illinois at Urbana-Champaign, Urbana, IL 61801-3080, USA*

<sup>2</sup>*Department of Physics, The Pennsylvania State University, University Park, Pennsylvania 16802, USA*

(Dated: February 13, 2025)

## EXPERIMENTAL METHODS

### Preparation of initial Bose-Einstein condensate

Our experimental procedure begins by collecting roughly  $10^8$  rubidium-87 atoms in a magneto-optical trap and cooling them by D<sub>2</sub> optical molasses. We then optically pump the atoms to the  $|F, m_F\rangle = |1, -1\rangle$  ground state of the  $5S_{1/2}$  manifold and load them into a magnetic quadrupole trap with a gradient of 130 G/cm along the axial, vertical direction. After 4.5 s of microwave-based evaporation, we load  $\sim 10^6$  atoms into a hybrid trap consisting of crossed optical dipole trap beams (with respective wavelengths of 1064 nm and 1070 nm) and a weak magnetic gradient of 28 G/cm. Finally, 12 s of forced optical evaporation in the hybrid trap results in a nearly pure Bose-Einstein condensate (BEC) of  $8(2) \times 10^4$  atoms confined in a trap with measured harmonic frequencies  $\{\omega_x, \omega_y, \omega_z\} = 2\pi \times \{130, 85, 30\}$  Hz. The frequency along the  $z$ -axis, which is along the direction of the Bragg excitation, is measured directly by dipole oscillations of the atoms. The frequencies along  $x$  and  $y$  are measured based on trap-loss spectroscopy by modulating the intensity of the trap laser beams.

The interference of the 1064 nm hybrid trap beam with a second, counter-propagating 1064 nm beam allows us to perform Bragg excitations of the atoms. We use a combination of arbitrary waveform generation and rf amplitude control via a voltage variable attenuator to control the relative frequency and the individual intensities of the interfering Bragg laser beams.

### Two-photon Bragg transition

Two-mode quantum gases are prepared in the momentum basis via excitation of a single Bragg resonance of the <sup>87</sup>Rb condensate atoms using two counter-propagating laser beams having wavelength  $\lambda = 1064$  nm. Bragg excitation involves the pairwise off-resonant absorption-stimulated emission of photons from a pair of laser fields. In our case, the two laser fields are directly counter-propagating, with photons from each field possessing momentum  $\hbar k = h/\lambda$ , such that a total momentum of  $2\hbar k$  is transferred to the atoms in a Bragg scattering process. The Bragg scattered atoms possess a kinetic energy of  $(2\hbar k)^2/2m = 4E_r$ , with  $m$  the atomic mass and  $E_r$  the recoil energy associated with an atom possessing a single

photon momentum ( $\hbar k$ ).

We prepare our two-mode gases by laser-dressing of the +1st Bragg resonance involving the momentum modes  $|0\hbar k\rangle$  and  $|2\hbar k\rangle$  (labeled by their characteristic momentum along the direction of Bragg excitation). In the lab frame and at the single-particle level, these two modes differ in energy by  $4E_r = h \times 8.111$  kHz. Resonant Bragg excitation between the modes  $|0\hbar k\rangle$  and  $|2\hbar k\rangle$  occurs when the difference frequency of the Bragg lasers is matched to this condition. This is associated with an optical potential moving at a velocity  $v_L = (4E_r/\hbar)/(2k) = \hbar k/m$  relative to the at rest condensate. To note, other first-order Bragg resonances (such as  $|2\hbar k\rangle \leftrightarrow |4\hbar k\rangle$  and  $|-2\hbar k\rangle \leftrightarrow |0\hbar k\rangle$ ) are separated in frequency by  $8E_r/h \approx 16.2$  kHz, and the  $|0\hbar k\rangle \leftrightarrow |2\hbar k\rangle$  transition can be isolated by restricting the potential depth of the moving standing wave to be much less than  $8E_r$ . This equivalently relates to the Bragg Rabi rate associated with the  $|0\hbar k\rangle \leftrightarrow |2\hbar k\rangle$  transition being small compared to  $2\pi \times 16.2$  kHz.

### Bragg parameter determination and calibration

The coupling rate, or Bragg Rabi rate,  $J$  of the Bragg field on resonance is calibrated by measuring the oscillatory population dynamics of the discrete momentum modes having momenta  $0\hbar k$  and  $2\hbar k$ . We apply approximately square Bragg pulses and measure the fraction of atomic population transferred between two momentum modes as a function of pulse duration. We measure sinusoidal Rabi oscillations of the mode populations, directly calibrating the Bragg coupling rate  $J$  (for large  $J$ ) by comparison to simulations of a simple coupled two-mode system. The detuning  $\delta$  of the Bragg field away from single-particle resonance is based on direct knowledge of the relative laser frequency.

### Calibration of the mean-field interaction strength

Based on the measured atom number of  $8(2) \times 10^4$  (with the quoted uncertainty relating solely to statistical shot-to-shot atom number fluctuations, ignoring larger systematic uncertainty based on our absorption imaging analysis), the measured harmonic trapping frequencies, and the known properties of <sup>87</sup>Rb atoms, we can estimate a trap-averaged mean-field interaction strength of

our initial ( $|0\hbar k\rangle$ ) condensates of  $\bar{U} = 590(60)$  Hz [1]. This simple estimate ignores the enhanced confinement of the small magnetic quadrupole potential.

We can experimentally calibrate the mean-field interaction strength by performing Bragg spectroscopy [2, 3]. We assume the  $2\hbar k$  mode to be perfectly distinguishable from the initial  $0\hbar k$  condensate mode, which in the linear response regime will lead to an added collective frequency shift of  $U$  to Bragg transition for atoms transferred to the  $2\hbar k$  mode, stemming from exchange interactions with the condensate. This ideal shift of  $U$  (with  $\hbar U = g\rho$  the mean-field energy) is strictly true for  $2k\xi \gg 2\pi$  [ $\xi \gg \lambda/2$ ], with  $\xi = (8\pi\rho a_s)^{-1/2} = (\hbar/(2mU))^{1/2}$  the healing length, and this (not entirely valid) assumption should lead to a slight underestimation of the mean-field energy. Similar to Ref. [4], we apply weak Bragg pulses ( $2\pi \times 250$  Hz Rabi rate, duration of  $400 \mu\text{s}$ ) and measure the fraction of atoms transferred out of the  $0\hbar k$  condensate as a function of the two-photon detuning. Averaging over the response observed for the +1st ( $|0\hbar k\rangle \leftrightarrow |2\hbar k\rangle$ ) and -1st ( $|0\hbar k\rangle \leftrightarrow |-2\hbar k\rangle$ ) Bragg transitions, and accounting for deviations from the linear response regime by comparing to simple two-mode simulations, we estimate a trap-averaged mean-field energy  $\bar{U}/2\pi \approx 0.9(1)$  kHz. This measured value (which is an underestimate due to the ignored effects of screening) is larger than the value estimated solely from the measured atom number and trap frequencies. This disagreement likely stems from a systematic underestimation of the atom number based on our absorption imaging analysis.

The value of  $\bar{U}/2\pi = 860$  Hz that is used throughout the main text is based purely on finding the value that gives the best global agreement between the ground state (GS) magnetization response data and the theory curves based on three-dimensional Gross-Pitaevskii equation (3D-GPE) simulations, as shown in Fig. 2 of the main text. The quoted value of  $\bar{U}$  for the simulations reflects the trap-averaged mean-field shift of the initial density distribution, prior to any Bragg dynamics.

### Preparation of the Bragg-dressed states

As discussed in the main text, we prepare our Bragg-dressed states by a relatively rapid but smooth ramping procedure. We first prepare dressed states in the “large-field” limit, where the total strength of the Bragg field,  $\sqrt{\delta^2 + 4J^2}$  is kept large relative to the scale of collective interactions,  $\bar{U}$ , via a two-step process lasting 2 ms.

We begin with atoms in the mode  $|0\hbar k\rangle$  and with a detuning  $\delta_i$  from the  $|0\hbar k\rangle \leftrightarrow |2\hbar k\rangle$  Bragg resonance that is relatively large ( $2\pi \times \pm 5.8$  kHz for the excited/ground state preparation) but still far from addressing any of the neighboring Bragg resonances to the states  $|-2\hbar k\rangle$  or  $|4\hbar k\rangle$ . With this large detuning fixed, we first smoothly ramp up the Bragg coupling rate  $J$  over 1 ms to its max-

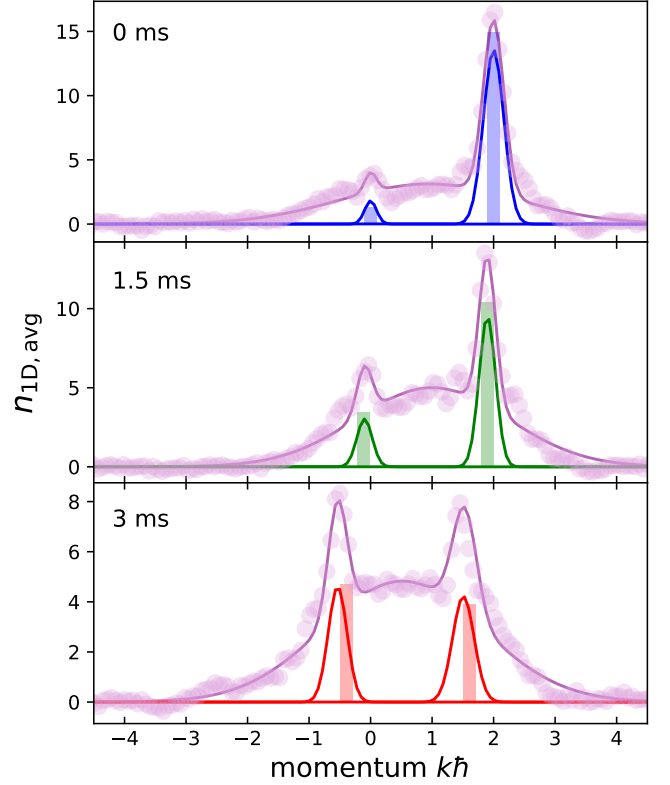

FIG. S1: **Trap-induced evolution of the Bragg-dressed ground state.** Data (faint purple circles) are the averaged (over 20 images) integrated optical density profiles with fit-resolved mode peaks for  $2\hbar k$  and  $0\hbar k$  of the prepared dressed ground state (GS). All panels reflect GS data taken at a final Bragg detuning of  $\delta_f/2\pi = 2.9$  kHz, with 2 ms of state preparation. The top, middle, and bottom panel respectively relate to holding at  $J_f = J_{max}$  for 0, 1.5, and 3 ms after state preparation (i.e., the same hold times as in the main text Fig. 2 inset). The faint bars show the (scaled) amplitudes and positions of the discretized momentum orders from corresponding 3D-GPE simulations based on the same state preparation and holding protocol (as described further and shown in Fig. S4).

imal value  $J_{max} = 2\pi \times 1.57(4)$  kHz. Then, in the second step of the preparation, the Bragg field detuning is smoothly swept (with a two-point cubic spline profile) to a chosen final value of  $\delta_f$  over a duration of 1 ms.

### Evolution of the Bragg-dressed states in the trap

After the initial state preparation and near resonance, the atoms are essentially in a coherent state superposition of the modes  $|0\hbar k\rangle$  and  $|2\hbar k\rangle$ . We find in experiment that the Bragg-dressed ground state can survive (with distinct

diffraction peaks) for several seconds in our hybrid trap (for  $\delta = 0$  and  $J = J_{max}$ ). This lifetime is much longer than the additional 3 ms we employ to ramp down  $J$  so as to probe the properties of the Bragg-dressed states under increasing  $\bar{U}/J$  ratios.

Due to the non-zero center-of-mass (COM) and the presence of the hybrid trapping potential, the Bragg-dressed state does evolve and undergo apparent dipole oscillations in the trap after it is prepared. At short times, the dressed state with mean initial velocity  $\bar{v}_i = \hbar k/m$  is observed (in experiment and in the 3D-GPE simulations) to evolve in mean velocity as  $\bar{v}(t) \approx \bar{v}_i \cos(\omega t)$ . Because of the presence of the coherent Bragg coupling beams, we continue to observe two diffraction peaks separated in momentum by  $2\hbar k$ , which move together as the dressed state is slowed down by the trapping potential, as shown in Fig. S1. To note, we refer to the discrete momentum orders as  $|0\hbar k\rangle$  and  $|2\hbar k\rangle$ , despite their translation to different momentum values as they evolve in the trap. As the dressed state mean velocity changes, the atoms experience an effective added detuning away from the Bragg resonance condition (due to Doppler shifts), as the Bragg resonance depends on the mean velocity for two momentum states separated by  $2\hbar k$  [resonance condition occurring at a laser frequency detuning of  $4(E_r/\hbar)(m\bar{v}/\hbar k)$ ].

Because of this trap effect, by which the atoms experience a time-dependent change to their Bragg resonance condition as the dressed states evolve in the trap, we choose to have our final experimental step (a rampdown of the Bragg coupling to explore the states in the  $\bar{U} \sim J$  limit) be short compared to a quarter trap period along the direction of the Bragg excitation ( $T_z/4 \approx 8.3$  ms). However, we still wish to perform a slow, adiabatic ramp so that the dressed atomic GS and ES may evolve quasi-adiabatically as the  $U/J$  ratio is increased. We choose a duration of 3 ms as a compromise between being too fast for the interactions to play an important role and being too slow such that the trap force significantly alters the dressed state. For this duration of our  $J$  rampdown, we find in the main text that the trap-shifted resonance condition ( $\mathcal{M}_{GS} = 0$ ) appears at  $\delta_f \approx 2.3$  kHz, consistent with the expected evolution of  $\bar{v}$  is one accounts for some evolution during the first 2 ms of state preparation.

### Rampdown of $J$ to $J_f$

In the final stage of the experiment prior to measurement, we perform a smooth 3 ms ramp down fo the Bragg coupling amplitude from our maximum value  $J_{max}$  to a variable final value  $J_f$ . We observe that, while fundamentally non-optimal due to the time constraints imposed by evolution in the trap, this rampdown duration is sufficient to observe strong apparent symmetry breaking of the dressed ground state (GS) under resonant, low coupling amplitudes. In the main text, we use this three-

stage sequence (with parameters varied according to the dashed lines in Fig. 1 of the main text) to explore the behavior of the dressed GS and the excited state (ES) within the parameter space of this coupled two-level system, varying  $J_f$  and  $\delta_f$ .

### Measurement and Image Processing

Following the preparation of our Bragg dressed states and ramping to a final  $J_f$  value, we release the atoms by turning off the Bragg lasers, the quadrupole trap, and the optical trapping beams. After a 20 ms-long time-of-flight, we perform absorption imaging of the atomic momentum distribution. The resulting primary data consists of cropped 200 pixel  $\times$  50 pixel absorption images.

Initial processing of the image datasets involves an integration on the  $y$ -axis (transverse to the direction of the Bragg excitation) to obtain 200-element data arrays. We conduct a background subtraction by taking the average of a left-tail 20-pixel mean-value and a right-tail 20-pixel mean-value (with these regions containing no atoms) and subtracting the resulting value from the array. We loosely filter our data based on the integrated atom number of these images, with the quoted atom number of  $8(2) \times 10^4$  reflecting the atom number after this filtering. This quoted atom number is based on Gaussian fitting of the integrated optical density, converting to atom number by dividing through by the full resonant cross section (which likely leads to a slight underestimate of the true atom number).

### Multi-Gaussian fitting analysis and determination of $\mathcal{M}$ for the GS and ES

To analyze the dressed state momentum profiles (as depicted in Fig. 3 of the main text), we fit them with a multi-peak Gaussian function. The fits are performed within OriginPro 2024 using the Multiple Peak Fit analysis tool. For the GS, the integrated weights under the narrow momentum peaks associated with the coherent diffraction orders are used to determine the discrete momentum mode populations.

As described in the main text, we define the “magnetization”  $\mathcal{M}$  of the dressed states ( $\propto \langle \hat{S}_z \rangle$ ) that characterizes the degree of population imbalance in the two-mode system. The experimental determination of  $\mathcal{M}$  is different for the GS and ES, reflecting the qualitative differences observed for their respective momentum profiles. After state preparation and for large  $J$ , the GS and ES appear similar, with coherent diffraction peaks on top of a broad background component (a combination of residual thermal atoms and atoms scattered from the coherent peaks due to  $s$ -wave scattering during time of flight). However, for smaller values of  $J_f$  and near the

trap-shifted resonance condition, the ES only exhibits a single, rather broad momentum component while the GS continues to display coherent momentum peaks on top of a low, broad background.

The GS magnetization is determined by the difference of the normalized populations within the two narrow diffraction components at  $2\hbar k$  and  $0\hbar k$ , namely  $\mathcal{M}_{\text{GS}} = P_2 - P_0$  (with  $P_2 + P_0 = 1$ , not including the contribution of atoms from the low, broad background). For the ES, due to the general lack of distinct momentum modes at  $0\hbar k$  and  $2\hbar k$ , we use an alternative definition of  $\mathcal{M}$ . Specifically, we extract the normalized imbalance of atoms having momentum above and below  $1\hbar k$ ,  $\mathcal{M}_{\text{ES}} = P_{>1} - P_{<1}$  (with  $P_{>1} + P_{<1} = 1$ ). For this determination, we calibrate the momentum axis of the ES (specifically, the  $1\hbar k$  position) by the positions of the GS momentum profile for the identical ramping protocol.

## THEORETICAL MODELING

Here, we conduct a theoretical investigation of our system from the point of view of a harmonically-confined Bose-Einstein condensate evolving under a traveling-wave optical potential generated by our Bragg fields. Our investigation consists of an analysis of three fundamental models: the many-body two-mode model as presented in Eq. 1 of the main text, its classical (large- $N$ ) limit, and the three-dimensional real-space Gross-Pitaevskii model (3D-GPE). In this section, we consider the first two of these, which fundamentally ignore effects and influences relating to the trapping potential (inhomogeneous density, in-trap dynamics, etc.). Later on we separately discuss our real-space modeling based on the 3D-GPE simulations.

Both the many-body two-mode model and its classical variant allow us to understand the idealized dynamics of the two-mode condensate with coherent inter-mode coupling (or tunneling), bias potentials (differences of the mode-dependent single-particle energies), and mode-dependent interactions. These models can be derived from the full, second-quantized Hamiltonian

$$\hat{H} = \hat{H}_0 + \hat{V}_{\text{lat}} + \hat{V}_{\text{int}} \quad (\text{S.1})$$

where the terms take the form

$$\hat{H}_0 = \int d^3\mathbf{r} \hat{\Psi}^\dagger(\mathbf{r}) \left[ -\frac{\hbar^2}{2m} \nabla^2 + \sum_{\sigma \in \{x,y,z\}} \frac{1}{2} m \omega_\sigma^2 \sigma^2 \right] \hat{\Psi}(\mathbf{r}) \quad (\text{S.2})$$

$$\hat{V}_{\text{lat}} = \int d^3\mathbf{r} \hat{\Psi}^\dagger(\mathbf{r}) \left[ 2\hbar J \cos(2\mathbf{k}_r \cdot \mathbf{r} - \omega t) \right] \hat{\Psi}(\mathbf{r}) \quad (\text{S.3})$$

$$\hat{V}_{\text{int}} = \frac{g}{2} \int d^3\mathbf{r} \hat{\Psi}^\dagger(\mathbf{r}) \hat{\Psi}^\dagger(\mathbf{r}) \hat{\Psi}(\mathbf{r}) \hat{\Psi}(\mathbf{r}) \quad (\text{S.4})$$

where  $\omega_\sigma$  is the trapping frequency in direction  $\sigma$  for a harmonic potential acting on an atom at position  $\mathbf{r}$ ,  $J$

is the coupling strength, and  $g$  is the boson-boson scattering strength.  $\hat{\Psi}^\dagger(\mathbf{r})$  creates a complex scalar boson at position  $\mathbf{r}$  and satisfies the bosonic commutation relations

$$[\hat{\Psi}(\mathbf{r}), \hat{\Psi}^\dagger(\mathbf{r}')] = \delta^3(\mathbf{r} - \mathbf{r}'). \quad (\text{S.5})$$

We neglect losses to collisions with thermal components of the gas so that the total number of atoms in the condensate is conserved

$$\hat{N} = \int d^3\mathbf{r} \hat{\Psi}^\dagger(\mathbf{r}) \hat{\Psi}(\mathbf{r}). \quad (\text{S.6})$$

The interaction term  $V_{\text{int}}$  describes the low energy s-wave collisions between the  $^{87}\text{Rb}$  atoms. It is scaled by the interaction parameter,  $g$ , which in turn is proportional to the s-wave scattering length  $a_s$ , given as

$$g = \frac{4\pi\hbar^2 a_s}{m}. \quad (\text{S.7})$$

To derive a simplified model which considers only the two modes of interest, we write  $\hat{\Psi}(\mathbf{r})$  in terms of momentum-basis creation and annihilation operators

$$\hat{\Psi}(\mathbf{r}) = \sum_{\mathbf{k}} \hat{a}_{\mathbf{k}} e^{i\mathbf{k} \cdot \mathbf{r}}. \quad (\text{S.8})$$

Then the interaction  $\hat{V}_{\text{int}}$  takes the form

$$\hat{V}_{\text{int}} = \frac{g}{2\mathcal{V}} \sum_{\mathbf{k}, \mathbf{k}', \mathbf{q}} \hat{a}_{\mathbf{k}+\mathbf{q}}^\dagger \hat{a}_{\mathbf{k}'-\mathbf{q}}^\dagger \hat{a}_{\mathbf{k}'} \hat{a}_{\mathbf{k}} \quad (\text{S.9})$$

where  $\mathcal{V}$  is the volume occupied by the Bose gas (and where we express a form with explicit momentum conservation). In the following, we ignore the evolution of the modes  $\hat{a}_{\mathbf{k}}$  due to the trap and take the Bose gas to have uniform density  $\rho = N/\mathcal{V}$ . With these assumptions, the mean field energy of the condensate is  $\hbar U = g\rho$  and the single particle interaction strength is  $u = U/N = g/\mathcal{V}$ .

To derive the properties of the uniform or trapped Bose gas, one typically proceeds by assuming only the zero momentum mode  $a_0$  is macroscopically occupied. However, here we assume both the  $\mathbf{k} = 0$  and  $2\mathbf{k}_r$  modes are macroscopically occupied. To that end, we write (S.8) as

$$\hat{\Psi}(\mathbf{r}) = \hat{a}_0 + \hat{a}_{2\mathbf{k}_r} e^{i2\mathbf{k}_r \cdot \mathbf{r}}. \quad (\text{S.10})$$

With this ansatz, and ignoring the harmonic trapping potential, the terms of the Hamiltonian (S.1) become

$$\hat{H}_0 = \epsilon_0 \hat{a}_0^\dagger \hat{a}_0 + \epsilon_{2\mathbf{k}_r} \hat{a}_2^\dagger \hat{a}_2 \quad (\text{S.11})$$

$$\hat{V}_{\text{lat}}/\hbar = J e^{-i\omega t} \hat{a}_2^\dagger \hat{a}_0 + J e^{i\omega t} \hat{a}_0^\dagger \hat{a}_2 \quad (\text{S.12})$$

$$\hat{V}_{\text{int}}/\hbar = u \hat{a}_0^\dagger \hat{a}_0 \hat{a}_2^\dagger \hat{a}_2 + u \hat{N}(\hat{N} - 1)/2 \quad (\text{S.13})$$

where we have rescaled the momentum-basis creation and annihilation operators  $\hat{a}_0 \rightarrow \sqrt{\mathcal{V}} \hat{a}_0$  and  $\hat{a}_{2\mathbf{k}_r} \rightarrow \sqrt{\mathcal{V}} \hat{a}_2$  so that the number operator is

$$\hat{N} = \hat{a}_0^\dagger \hat{a}_0 + \hat{a}_2^\dagger \hat{a}_2 \quad (\text{S.14})$$

We note that  $\epsilon_0 = 0$  and we drop terms proportional to  $\hat{N}$  as they are conserved quantities that do not contribute to the population dynamics.

We can transform the operators  $\hat{a}_0$  and  $\hat{a}_2$  into a time-dependent rotating frame by taking  $\hat{a}_0 \rightarrow e^{i\omega t/2}\hat{a}_0$  and  $\hat{a}_2 \rightarrow e^{-i\omega t/2}\hat{a}_2$ . We arrive at the effective two-mode, time-independent Hamiltonian and write  $\hat{H}_{\text{eff}} = \hat{H}_0 + \hat{V}_{\text{lat}} + \hat{V}_{\text{int}}$  as

$$\hat{H}_{\text{eff}}/\hbar = \frac{\delta}{2}(\hat{N}_0 - \hat{N}_2) + J(\hat{a}_2^\dagger \hat{a}_0 + \hat{a}_0^\dagger \hat{a}_2) + u\hat{N}_0\hat{N}_2 \quad (\text{S.16})$$

Importantly, this time-dependent transformation preserves the canonical equations of motion  $i\partial_t \hat{a} = [\hat{a}, \hat{H}]$ .

On resonance,  $\delta = 0$ , the model exhibits two phases separated by a critical value  $J_c = Nu/2 = U/2$ . Given  $N$  atoms in the condensate and  $J \gg J_c$ , the ground state

is unique and given simply by  $|\Psi_0\rangle = (2^{-N}N!)^{-1/2}(\hat{a}_0^\dagger + \hat{a}_2^\dagger)^N|\text{vac}\rangle$  where  $|\text{vac}\rangle$  is the bosonic vacuum. For  $J = 0$ , the ground state energy becomes doubly degenerate with ground states  $|\Psi_i\rangle = (N!)^{-1/2}(\hat{a}_i^\dagger)^N|\text{vac}\rangle$ ,  $i = 0, 2$ . That is, all atoms are found in one mode or the other. In this language, individual measurements of the magnetization  $\mathcal{M} = \langle \hat{N}_2 - \hat{N}_0 \rangle / N$  take on a non-zero value for  $J < J_c$ .

At this stage, we can take the limit of large mode occupation  $N \rightarrow \infty$ . In this limit, the operators  $\hat{a}_j$  become c-numbers which we write as

$$\hat{a}_j(t) \rightarrow \sqrt{N}\chi_j(t) \quad (\text{S.17})$$

and are normalized so that  $|\chi_0(t)|^2 + |\chi_2(t)|^2 = 1$ . We then have the classical, two-mode GPE

$$i\partial_t \begin{pmatrix} \chi_0 \\ \chi_2 \end{pmatrix} = \begin{pmatrix} \frac{1}{2}(\delta + U(|\chi_2|^2 - |\chi_0|^2)) & J \\ J & -\frac{1}{2}(\delta + U(|\chi_2|^2 - |\chi_0|^2)) \end{pmatrix} \begin{pmatrix} \chi_0 \\ \chi_2 \end{pmatrix} \quad (\text{S.18})$$

The population dynamics of (S.16) can be elucidated by mapping it to that of a single spin with total spin  $S = N/2$ . This mapping allows us to visualize the behavior on the generalized Bloch sphere (Fig. 4 (d) of main text). The mapping takes the form

$$\hat{S}_z = \frac{1}{2}(\hat{N}_0 - \hat{N}_2) \quad (\text{S.19})$$

$$\hat{S}^+ = \hat{a}_0^\dagger \hat{a}_2 \quad (\text{S.20})$$

$$\hat{S}^- = \hat{a}_2^\dagger \hat{a}_0 \quad (\text{S.21})$$

so that Eq. S.16 becomes

$$\hat{H}_{\text{eff}}/\hbar = \delta \hat{S}_z + 2J \hat{S}_x - u \hat{S}_z^2. \quad (\text{S.22})$$

where  $u = U/N$ , also shown as Eqn. 1 in main text. The coherent spin states  $|\theta, \phi\rangle \equiv |\Omega\rangle$  are given by

$$|\Omega\rangle = (\cos(\theta/2))^{2S} \exp(\tan(\theta/2)e^{i\phi}\hat{S}^-)|S\rangle \quad (\text{S.23})$$

where  $\hat{S}_z|S\rangle = S|S\rangle$  is the fully polarized spin up state and corresponds to the  $|N_0 = 0, N_2 = N\rangle$  state in the boson picture [5]. The coherent spin states form an over complete basis on the sphere and can be used to construct the Husimi  $Q$  distribution

$$Q = \frac{1}{\pi} \langle \Omega | \rho | \Omega \rangle \quad (\text{S.24})$$

which can be interpreted as a genuine probability distribution over classical phase space [6].

The  $-\hat{S}_z^2$  term is a one-axis twisting interaction [7] that can give rise to dynamical squeezing in this two-mode system. Correspondingly, the presence of this term can lead

to correlated eigenstates of the many-body model (S.22), such as when the system is ramped beyond the vertex of the separatrix. This is consistent with the observation of bifurcated  $\mathcal{M}$  distributions presented in the main text.

### Spontaneous symmetry-breaking in the two-mode model

The two-mode model admits a classical interpretation in terms of the conjugate variables  $\phi$  and  $\mathcal{M}$ , the relative phase and population difference between the two momentum modes

$$\mathcal{M} = |\chi_2|^2 - |\chi_0|^2 \quad (\text{S.25})$$

$$\phi = \arg(\chi_2^* \chi_0). \quad (\text{S.26})$$

Using Eq. S.18, one can show that

$$\frac{d\mathcal{M}}{dt} = J\sqrt{1 - \mathcal{M}^2} \sin \phi \quad (\text{S.27})$$

$$\frac{d\phi}{dt} = -\frac{\delta}{2} - \frac{U}{2}\mathcal{M} - J\frac{\mathcal{M} \cos \phi}{\sqrt{1 - \mathcal{M}^2}} \quad (\text{S.28})$$

which obey the Hamiltonian equations of motion

$$\frac{d\phi}{dt} = \frac{\partial H}{\partial \mathcal{M}} \quad \frac{d\mathcal{M}}{dt} = -\frac{\partial H}{\partial \phi} \quad (\text{S.29})$$

with Hamiltonian

$$H = -\frac{\delta}{2}\mathcal{M} - \frac{1}{4}U\mathcal{M}^2 + J\sqrt{1 - \mathcal{M}^2} \cos \phi. \quad (\text{S.30})$$

In the thermodynamic limit, this classical Hamiltonian has the interpretation of the free energy of a statistical



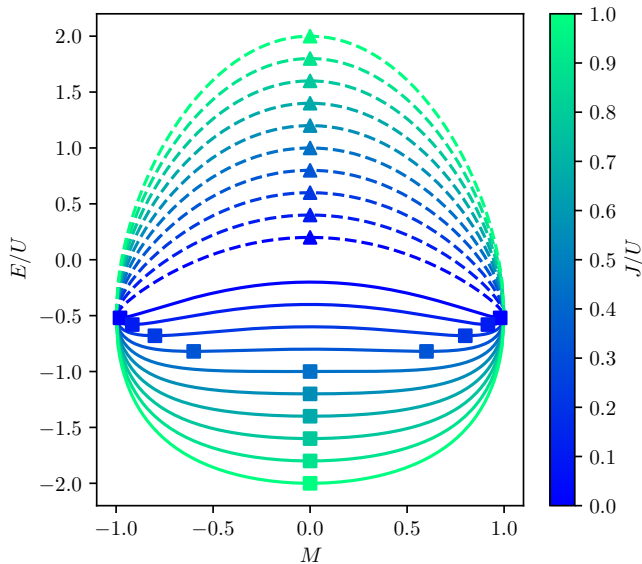

FIG. S2: **Ground state bifurcation.** Free energy of the two-mode model (Eq. S.30) on resonance ( $\delta = 0$ ) for the ground state (solid lines) and excited state (dashed lines). The global ground state(s) for particular values of  $J$  are indicated by squares and the highest excited states are indicated by triangles.

mechanical system with order parameter  $\mathcal{M}$ . This model provides some insight into why spontaneous symmetry-breaking occurs in the ground state ( $\phi = \pi$ ) and not in the excited state ( $\phi = 0$ ). The distinct behavior of these two cases are demonstrated in Fig. S2.

We see that a bifurcation occurs for the ground state curve when  $J < J_c = U/2$  which results in two degenerate ground states at  $\mathcal{M} = \pm\sqrt{1 - 4J^2/U^2}$  and an intermediate excited state at  $\mathcal{M} = 0$  in addition to the highest excited state for a total of four modes. On the other hand, above  $J_c$ , only one mode is present in each branch and thus the system contains only two modes. In this phase, the ground state branch is *paramagnetic* in that the equilibrium value of  $\mathcal{M}$  is proportional to the symmetry-breaking field  $\delta$ .

In this picture, spontaneous symmetry-breaking only occurs in the ground state branch because the bifurcation points emerge from the global ground state at  $\mathcal{M} = 0$  as  $J$  is lowered past  $J_c$ . The excited state is clearly unstable and is not infinitesimally connected to the new ground states. Thus, in the excited state, we expect to observe complicated dynamics as the system attempts to relax to the lowest energy state which is consistent with our observations, as seen in Fig. 3 (main text).

## NUMERICAL METHODS

To support our experimental work we performed numerical simulations using three distinct models: we simulated the full 3D GPE Eq. S.31 using the GPELab Matlab package [8], the two-mode GPE Eq. S.18, and the second-quantized Hamiltonian Eq. S.16 using the QuSpin Python package for exact diagonalization [9]. Specifically, we verified (1) the origin of the shift of the Bragg resonance by 2-3 kHz, (2) the efficacy of the much simpler two-mode model as a descriptor for the physics at hand, and (3) the quantum mechanical effects that govern the dynamical symmetry-breaking in the two momentum mode subspace.

### Numerically Capturing Symmetry-Breaking

To capture symmetry breaking in our models, we must account for quantum fluctuations associated with the occupation of each momentum mode. The 3D GPE, while an excellent tool for determining the bulk behavior of the condensate within the trap subject to the lattice potential, contains only information on the average occupation of each mode. To go beyond this mean field treatment, we explore the effect of fluctuations through (1) exact diagonalization of S.16 and (2) a truncated Wigner analysis of S.18 subject to local density approximation due to the inhomogeneous density profile of the gas induced by the harmonic trap.

Using exact diagonalization, we examined the spectrum and time-dependent behavior of Eq. S.16 for  $N = 50, 100$ , and  $500$  using  $U = \bar{U}$  and  $3\bar{U}/2$ . Although it is possible to obtain portions of the static spectrum for the realistic case of  $N = 8 \times 10^4$ , we were not able to perform a full time-dependent simulation using this value due to computational constraints. Fortunately, we maintain that this finite-sized analysis provides us with a qualitative understanding of the non-equilibrium dynamics of the condensate before and after the transition; this is because given a value of  $U$ ,  $J_c = U/2$  is fixed and independent of  $N$ . Thus, analyzing the behavior for finite  $N$  serves as a useful interpolation between the single-particle case and the thermodynamic limit, which is described by the 3D and two-mode GPE's.

Fig. S3 summarizes the results of these simulations. For  $J > J_c$ , the ground state is unique and maintains a large gap to the next excited state which allows adiabatic evolution throughout the ramp. However, upon sweeping past the phase transition at  $J = J_c$ , both numerical and experimental results deviated significantly from what one expects for a perfectly adiabatic sweep (i.e., from the ground state's response). Experimentally, this is demonstrated by the fact that  $g_{\text{res}}^{(2)}$  does not vanish as  $J_f \rightarrow 0$  and is corroborated by numerical results shown

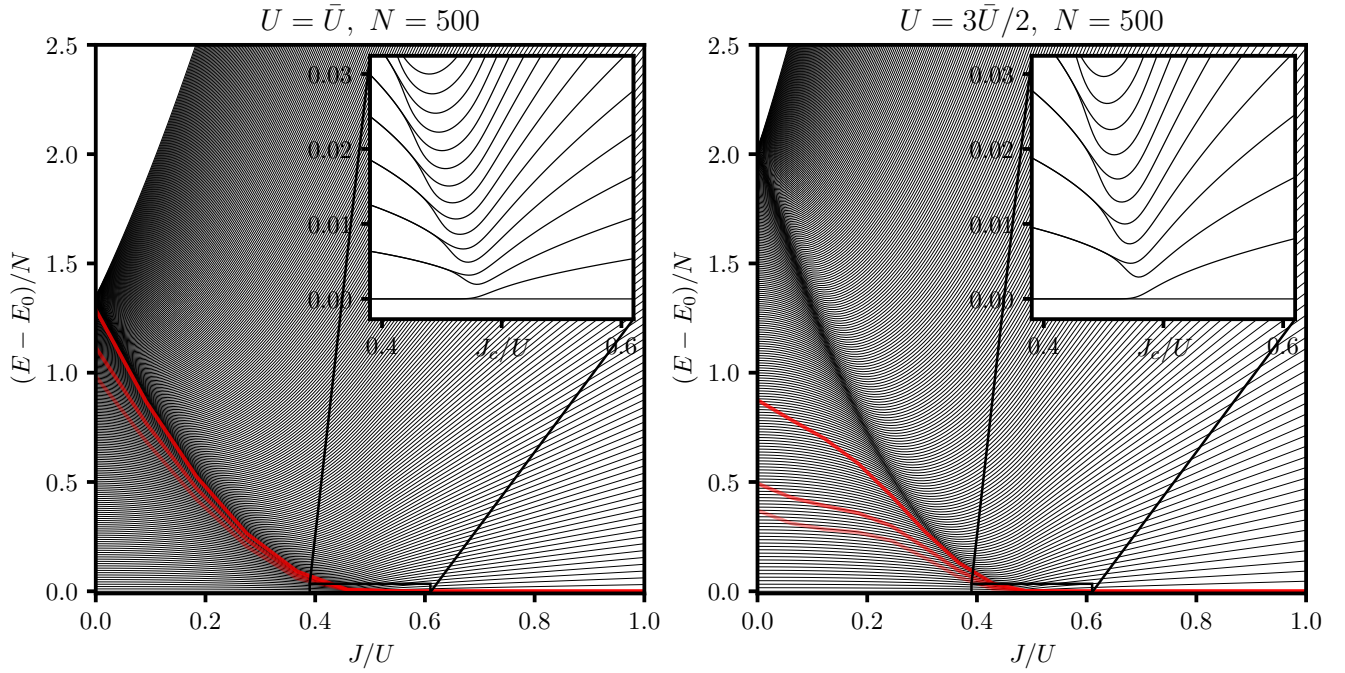

FIG. S3: **Diabatic state preparation.** Eigenstate energy spectrum of Eq. S.16 for  $N = 500$  for various values of  $J$ . Red curves are obtained by simulating the state preparation ramp assuming the system is in its ground state following the sweep of the detuning  $\delta$  for  $N = 50, 100, 500$  (increasing opacity). (Left) Excitation spectrum and time dependent energy expectation value using  $u = \bar{U}/N$  for various  $N$ . (Right), the same data but using an enlarged value of  $u = 3\bar{U}/2N$ . Note that only even levels for the energy spectrum are plotted in the underlying figure. This was done in order to make each curve more visible. (Inset) Excitation spectrum near the ground state quantum phase transition (QPT). Pairs of excited states in the paramagnetic phase merge and are squeezed together as  $J$  is tuned below  $J_c$  signaling a line of excited-state QPTs (ESQPTs). For any finite ramp time and a sufficiently large number of bosons, the effect of ramping  $J$  takes the system far from the ground state. This is consistent with the two-mode model in the thermodynamic limit, where the clustering of energy levels (ESQPTs) corresponds to the classical energy surfaces of Eq. S.30.

in Fig. S3. This is due to the finite ramp duration and the complicated level structure exhibited by Eq. S.16 at criticality; near  $J_c$ , previously well-separated even and odd parity states pair with one another resulting in a halving of the total number of non-degenerate states. In addition, the total spectrum is increasingly squeezed for increasing  $N$  so that as  $J$  is ramped below  $J_c$  at a finite rate, a series of Landau-Zener transitions carries the system away from the ground state (Fig. S3). This feature is clearly visible in the spectrum as a dark region where the spacing between levels becomes small. This effect is increasingly pronounced as  $N$  becomes large: the single particle excitation energy scales as  $u = \bar{U}/N$ . Thus, when the tunneling is ramped to  $J_f \approx 0$  over just 3 ms, the state prepared in the laboratory does not follow the true many-body ground state instead populating many low-lying energy states. This should result in a degree of symmetry-breaking that is less robust than that of the ground state, and this may explain why the experimental data does not show  $g_{res}^{(2)} \rightarrow 0$  as  $J_f \rightarrow 0$ .

To simulate the time-dependent dynamics (red curves),

we assumed that the initial state preparation procedure resulted in the ground state of Eq. S.16 for  $J > J_c$ .

To complement the finite-sized analysis, we also performed simulations of our system in the thermodynamic limit,  $N \rightarrow \infty$ , using the truncated Wigner approximation. The truncated Wigner approximation is valid near the thermodynamic limit where quantum fluctuations are relatively small and proceeds by evolving the classical equations of motion (Eq. S.18) for various initial conditions sampled from an initial Wigner distribution for the bulk system [10]. For each initial condition sampled from this distribution, we also independently sampled the interaction strength  $U$  from the Thomas-Fermi density profile. This is motivated by the fact that the local interaction strength is proportional to the local density at any point within the gas, and the simple two-mode model on its own ignores the inhomogeneous density. For all simulations of this form, we sampled  $10^4$  points.

We first assumed that the GS preparation protocol discussed in the main text resulted in a bosonic coherent

state

$$|\alpha_0, \alpha_2\rangle = e^{\alpha_0 \hat{a}_0^\dagger - \alpha_0^* \hat{a}_0} e^{\alpha_2 \hat{a}_2^\dagger - \alpha_2^* \hat{a}_2} |\text{vac}\rangle. \quad (\text{S.31})$$

This is equivalent to the initial state assumed in our exact diagonalization simulations in the limit  $N \rightarrow \infty$ . Since total atom number is conserved, we have  $|\alpha_0|^2 + |\alpha_2|^2 = N$ . Further, in the limit  $N \gg 1$ , each point in the classical  $(\mathcal{M}, \phi)$  phase-space can be identified with a unique coherent state with the mapping

$$\begin{aligned} \alpha_0 &= \sqrt{N \left( \frac{1 - \mathcal{M}}{2} \right)} \\ \alpha_2 &= \sqrt{N \left( \frac{1 + \mathcal{M}}{2} \right)} e^{i\phi}. \end{aligned} \quad (\text{S.32})$$

With this in mind, we instead write  $|\alpha_0, \alpha_2\rangle = |\mathcal{M}, \phi\rangle$ .

To simulate the symmetry-breaking dynamics associated with the ramp down of the inter-mode coupling  $J$ , we drew initial states  $(\mathcal{M}_0, \phi_0)$  from the probability distribution

$$\begin{aligned} P_{\text{coher}}(\mathcal{M}, \phi) &= |\langle \mathcal{M}, \phi | 0, \pi \rangle|^2 \\ &\approx \frac{1}{2\pi \sqrt{\sigma_{\mathcal{M}} \sigma_{\phi}}} e^{-\mathcal{M}^2/2\sigma_{\mathcal{M}}^2 - \phi^2/2\sigma_{\phi}^2} \end{aligned} \quad (\text{S.33})$$

where  $\sigma_{\mathcal{M}} = \sqrt{2/N}$  and  $\sigma_{\phi} = \sqrt{1/N}$ . The approximation is a result of the large- $N$  limit and an application of Laplace's method.

The dotted line of Fig. 4(d) of the main text was generated by numerically evaluating the trajectories with initial conditions sampled from  $P_{\text{coher}}$  according to Eq. S.18 and using our estimated atom number  $N = 8 \times 10^4$  and sampling independently the mean field energy  $U$  from a Thomas-Fermi density distribution with mean  $\bar{U} = 2\pi \times 0.86$  kHz. This however, was not sufficient to capture the degree of symmetry-breaking witnessed experimentally.

As discussed in the main text, this disagreement could be a result of (1) an underestimate of the average mean field energy, (2) the influence of parameter variations or experimental noise, or (3) a result of motion in the trap (including domain formation) which necessitates the treatment of more than two momentum modes. Staying within the two-mode picture for now, we addressed (1) by repeating the same analysis described above, but instead drawing  $U$  from a Thomas-Fermi distribution with mean  $1.5\bar{U}$  which corresponds to the dashed line in Fig. 4(d) of the main text. We addressed (2) by instead keeping the mean-field energy distribution fixed and enlarging the phase space distribution by taking  $\sigma_{\mathcal{M}} = 0.15$  and  $\sigma_{\phi} = 0.15\sqrt{2}$ , which corresponds to the solid line in Fig. 4(d) of the main text.

### 3D GPE Description of Momentum-State Lattices

The time-dependent Gross-Pitaevskii equation describes the real-space evolution of an interacting BEC. To simulate the behavior of our two-mode condensate, we employ a theoretical description of synthetic momentum-state lattices with a 3D Gross-Pitaevskii equation (GPE) to capture the effects of our external trapping potential as well as the many-body interaction. This treatment captures both the evolution of the state and real-space dynamics present in our experimental observations. The momentum-state lattice is developed from a weakly-trapped BEC interacting with two counterpropagating Bragg laser beams. The time evolution of the mean-field wavefunction is described by the Gross-Pitaevskii equation

$$i\hbar \partial_t \Psi = \left( -\frac{\hbar^2}{2m} \nabla^2 + V_{\text{trap}} + V_{\text{lat}} + g|\Psi|^2 \right) \Psi \quad (\text{S.31})$$

We approximate our hybrid trapping potential as a simple 3D harmonic oscillator potential

$$V_{\text{trap}} = \frac{1}{2} m (\omega_x^2 x^2 + \omega_y^2 y^2 + \omega_z^2 z^2) \quad (\text{S.32})$$

with  $\{\omega_x, \omega_y, \omega_z\} = 2\pi \{130, 85, 30\}$  Hz being our measured trap frequencies and  $m$  being the particle mass. The moving optical potential formed by the interfering Bragg laser beams is accounted for by the lattice

$$V_{\text{lat}} = 2\hbar J \cos(2kz + \phi(t)) \quad (\text{S.33})$$

where  $J$  is our Bragg coupling amplitude. The mathematical form of the detuning ( $\delta$ ) ramp is defined via the time-dependent lattice phase

$$\phi(t) = \phi_R + \int_0^t \delta(\tau) d\tau. \quad (\text{S.34})$$

Here  $\phi_R = \delta_R t$  relates to the single particle Bragg resonance with  $\delta_R = 4E_r/\hbar \approx 8.111$  kHz, while  $\delta(\tau)$  in the integral indicates the ramp of the detuning shown in Fig. 1 in the main text.

We use the open source GPELab MatLab package [8] to simulate the real-space dynamics, supplemented by fast Fourier transforms (FFTs) within MatLab to access momentum distributions. We initialize the beginning  $\Psi$  by imaginary time evolution, setting the non-linearity so that the trap-averaged mean-field interaction (prior to any Bragg-driven dynamics) is matched to  $\bar{U} = 2\pi \times 860$  Hz. We program our ramp sequence with the relevant time-dependent detuning  $\delta(t)$  and Bragg coupling  $J(t)$ . Finally, we obtain the density distribution of the final condensate wave function for chosen values of final detuning  $\delta_f$ . We do not directly model the time-of-flight expansion, but rather we conduct a Fourier



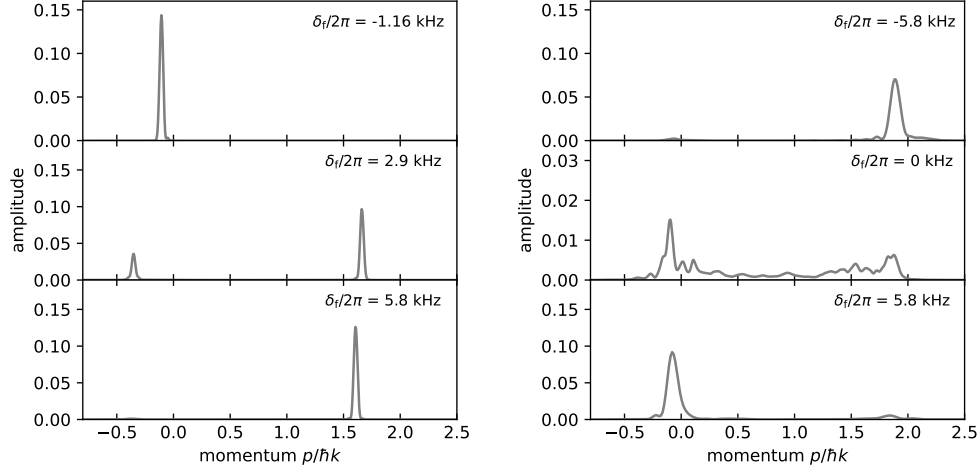

FIG. S4: **3D GPE simulations of the Bragg-dressed ground state (GS, left) and excited state (ES, right).** Momentum profiles of the GS (left column plots) and excited state ES (right column plots) resolved after simulating the state preparation procedure based on the real-space 3D Gross-Pitaevskii equation (GPE) as described in the supplementary text, also including the rampdown of the Bragg coupling to  $J_f = 0$ . For the GS ( $\delta_i/2\pi = -5.8$  kHz) and ES ( $\delta_i/2\pi = +5.8$  kHz), respectively, the vertical panels show the simulated momentum profiles for different final detuning values,  $\delta_f$ . As described in the text, the simulations assume a trap-averaged mean-field interaction of the initial condensate of  $\bar{U} = 2\pi \times 860$  Hz as well as a 3D harmonic trapping potential having trap frequencies  $\{\omega_x, \omega_y, \omega_z\} = 2\pi \times \{130, 85, 30\}$  Hz. There are two notable features of these plots based on (Fourier-transformed) real-space GPE simulations. First, while the major Bragg peaks appear at  $0\hbar k$  and  $2\hbar k$  at short times after the state preparation, the evolution of the Bragg-dressed states in the trapping potential cause them to migrate to other momentum values after the finite evolution time. Second, the ES profiles exhibit a highly broadened momentum distribution near Bragg resonance when  $J_f = 0$ , consistent with the distributions measured in experiment. We note that the simulations are based on Fourier transforms of the real-space distributions after the in-trap evolution, with no explicit consideration of the time-of-flight expansion (furthermore, there is no mechanism in the GPE simulations to induce the  $s$ -wave scattering halos that appear in the experimental profiles).

analysis on the final wave function after the 5 ms-long ramp protocol (for experiments with the full 3 ms ramp of  $J$ ) to generate momentum-space distributions. For the GS cases, discrete momentum mode populations (as depicted in Fig. S1) are found by integrating the distributions over windows in momentum space centered at the apparent diffraction orders. This mirrors the analysis in Ref. [11]. These mode populations are used to extract the GS magnetization,  $\mathcal{M}_{\text{GS}}$ .

As in our experiments, the ramps that prepare the ES in our simulations can exhibit a significant broadening associated with the population of a large number of momentum states (leading to the lack of discrete momentum peaks). This is particularly the case near  $\delta_f = 0$ , as shown in Fig. S4, where we observe violent spreading in momentum space (associated with an instability of the interacting condensate). Thus, for the excited state magnetization curves, we determine  $\mathcal{M}_{\text{ES}}$  with the same procedure as used for the data. We calibrate the momentum axis along the direction of the Bragg excitation by defining  $1\hbar k$  as the midpoint between the two peaks of the GS distribution for the same ramp profile. We then determine the normalized populations above and below

$1\hbar k$  by numerical integration of the simulated momentum distributions, finally taking their difference as  $\mathcal{M}_{\text{ES}}$ .

\* [bdemarco@illinois.edu](mailto:bdemarco@illinois.edu)

† [bgadway@illinois.edu](mailto:bgadway@illinois.edu)

- [1] F. Dalfovo, S. Giorgini, L. P. Pitaevskii, and S. Stringari, *Rev. Mod. Phys.* **71**, 463 (1999).
- [2] J. Stenger, S. Inouye, A. P. Chikkatur, D. M. Stamper-Kurn, D. E. Pritchard, and W. Ketterle, *Phys. Rev. Lett.* **82**, 4569 (1999).
- [3] R. Ozeri, N. Katz, J. Steinhauer, and N. Davidson, *Rev. Mod. Phys.* **77**, 187 (2005).
- [4] F. A. An, E. J. Meier, J. Ang'ong'a, and B. Gadway, *Phys. Rev. Lett.* **120**, 040407 (2018).
- [5] J. M. Radcliffe, *Journal of Physics A: General Physics* **4**, 313 (1971).
- [6] J. Hall, S. Malzard, and E.-M. Graefe, *Phys. Rev. Lett.* **131**, 040402 (2023).
- [7] M. Kitagawa and M. Ueda, *Phys. Rev. A* **47**, 5138 (1993).
- [8] X. Antoine and R. Dubosq, *Computer Physics Communications* **185**, 2969 (2014).
- [9] P. Weinberg and M. Bukov, *SciPost Physics* **2**, 003 (2017).

- [10] A. Sinatra, C. Lobo, and Y. Castin, [Journal of Physics B: Atomic, Molecular and Optical Physics](#) **35**, 3599 (2002).
- [11] T. Chen, D. Xie, B. Gadway, and B. Yan, “A gross-pitaevskii-equation description of the momentum-state lattice: roles of the trap and many-body interactions,” (2021), [arXiv:2103.14205 \[physics.atom-ph\]](#).
